# Supplementary material for: A Modular Graph-Native Query Optimization Framework
Source: arXiv:2401.17786 source file (2024-12-12)
Supplement: Supplementary file 1 [file sec-appendix.tex]

\section{APPENDIX}

\label{sec:appendix}
\subsection{Queries and Execution Plans}
In this section, we delineate the execution plans for queries, emphasizing the proficiency of \gopt~in ascertaining the most efficient search order for the query execution.
First, we provide detailed case study on the LDBC queries, taking $BI_9$ as a representative example, to compare the execution plans optimized by \gopt~and Neo4j.
Then, we present the execution plans for queries $QC_{1\ldots 4(a|b)}$ which are designed to assess the effectiveness of cost-based optimization techniques.

\subsubsection{Case Study on LDBC Queries}

\begin{figure}[h!]
  \centering
  \includegraphics[width=\linewidth]{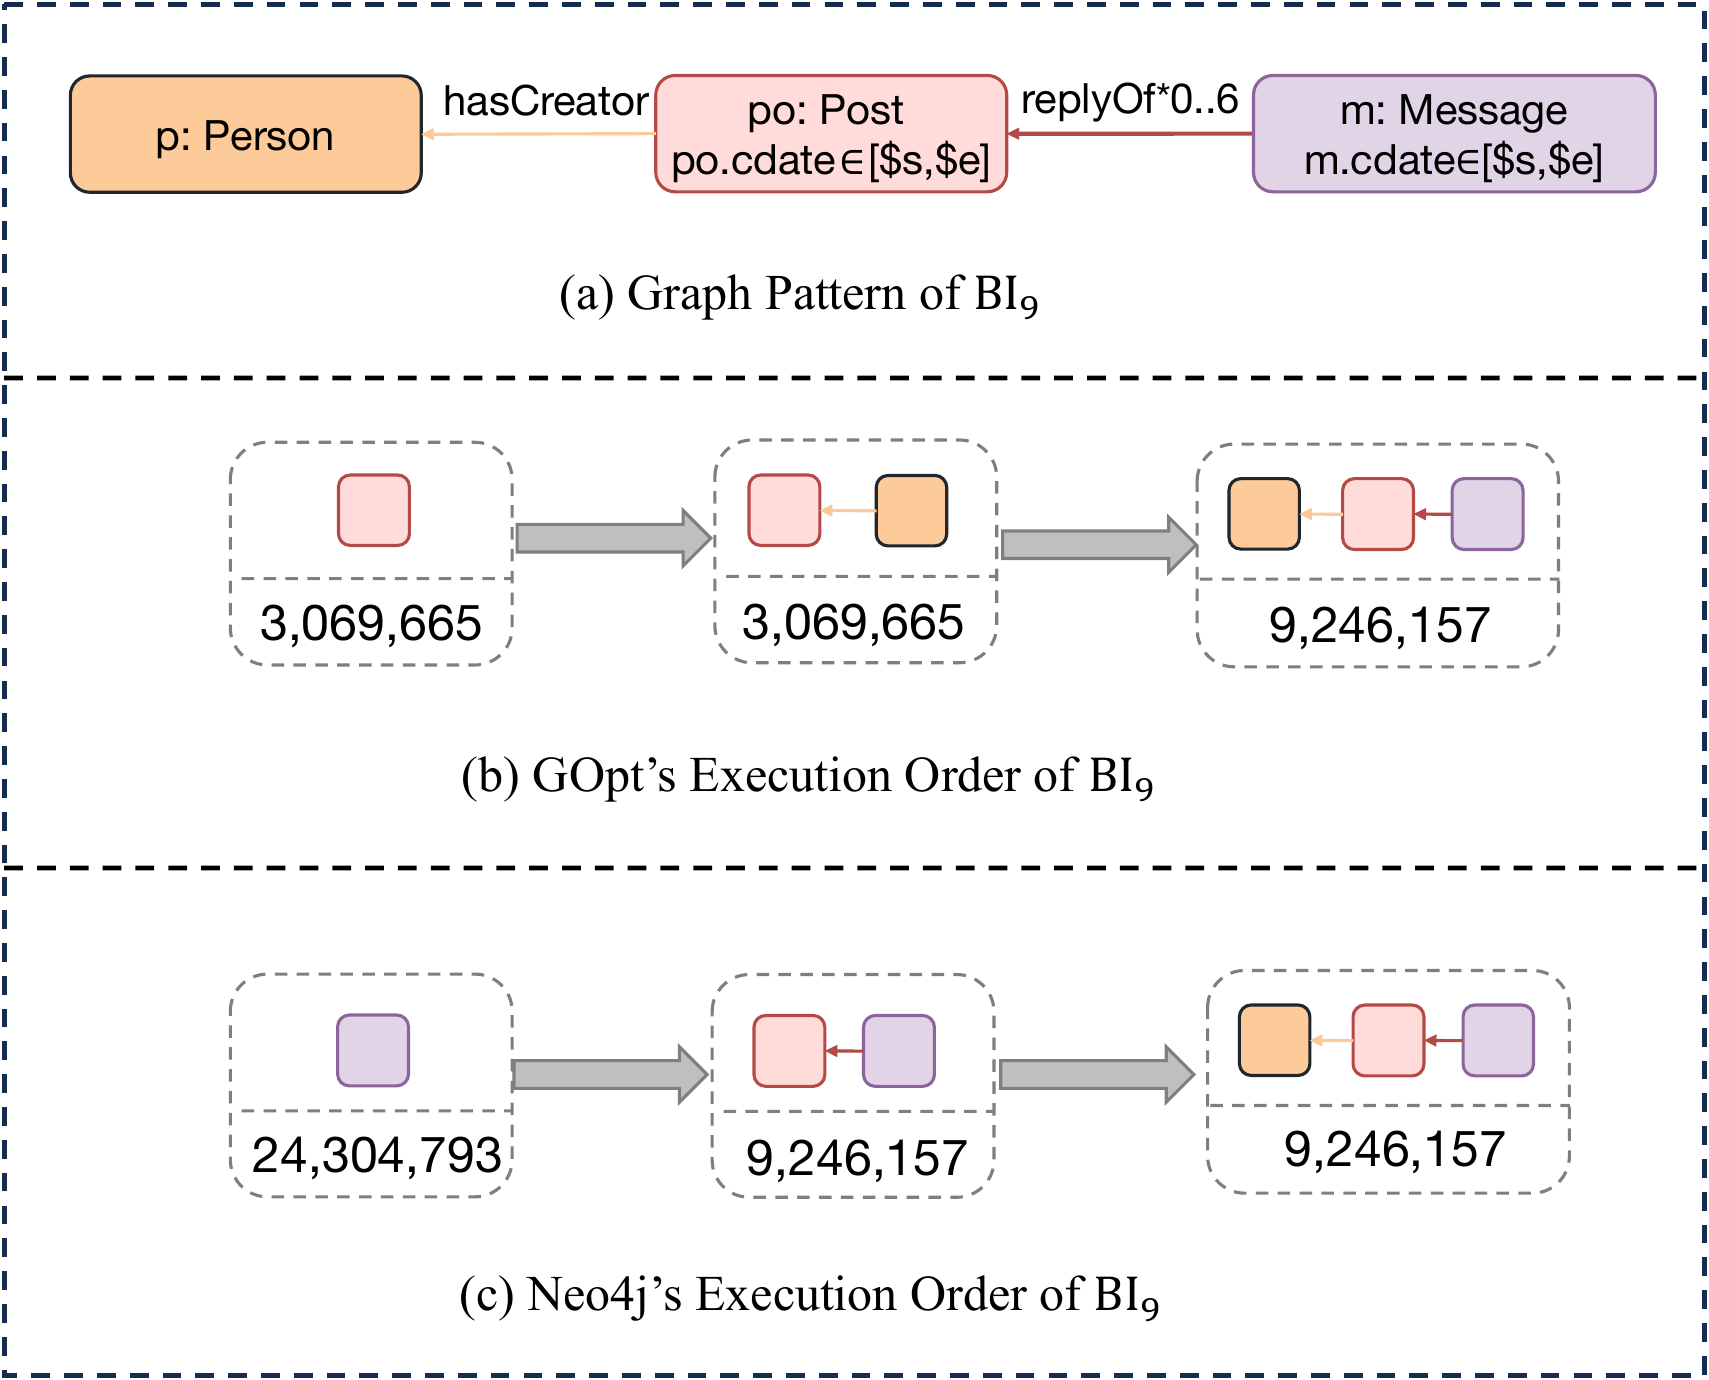}
  \caption{Execution Plans for $BI_9$}
  \label{fig:bi_plans}
\end{figure}

During our tests with the LDBC queries, \gopt~was observed to produce optimized plans that match the quality of manually optimized ones from prior research \cite{qian2021gaia}.
This case study take $BI_9$ on $G_{30}$ as an example to offer an in-depth comparison between the execution plans optimized by \gopt~and Neo4j.
The query is presented in \reffig{bi_plans}(a), and the execution order optimized by \gopt~and Neo4j are illustrated in \reffig{bi_plans}(b) and \reffig{bi_plans}(c), respectively.
For example, \gopt~starts the searching from \code{Post} $po$, while Neo4j starts from \code{Message} $m$.
We assessed both plans' performance, and illustrate the number of intermediate results produced during the query processing for each plan in \reffig{bi_plans}, highlighting that \gopt's plan generates merely $36\%$ of the intermediate results compared to Neo4j's, while being around $7.2\times$ faster as verified in the previous small-scale experiments.
% From the figure, we can see that the main reason for the performance gap is that Neo4j's plan results in an explosion of intermediate results, especially when expanding from \code{Person} $p_2$ (which has $76,561,414$ matchings) to \code{Message} $m_1$ (produced $73,852,535$ intermediate results) and $m_2$ (produced $26,100,505$ intermediate results). 
% In contrast, \gopt~expands $p_2$ from a user-specified starting point $p_1$, thereby limiting the number of potential matches for $p_2$ to $1,399$, and effectively minimizing the matching numbers for subsequent expansions to \code{Message} $m_1$ (limiting to $1,116,047$) and $m_2$ (limiting to $663,772$). 
This case study underscores \gopt's efficacy in optimizing the execution of complex queries.

\begin{figure*}[h!]
  \centering
  \includegraphics[width=0.9\linewidth]{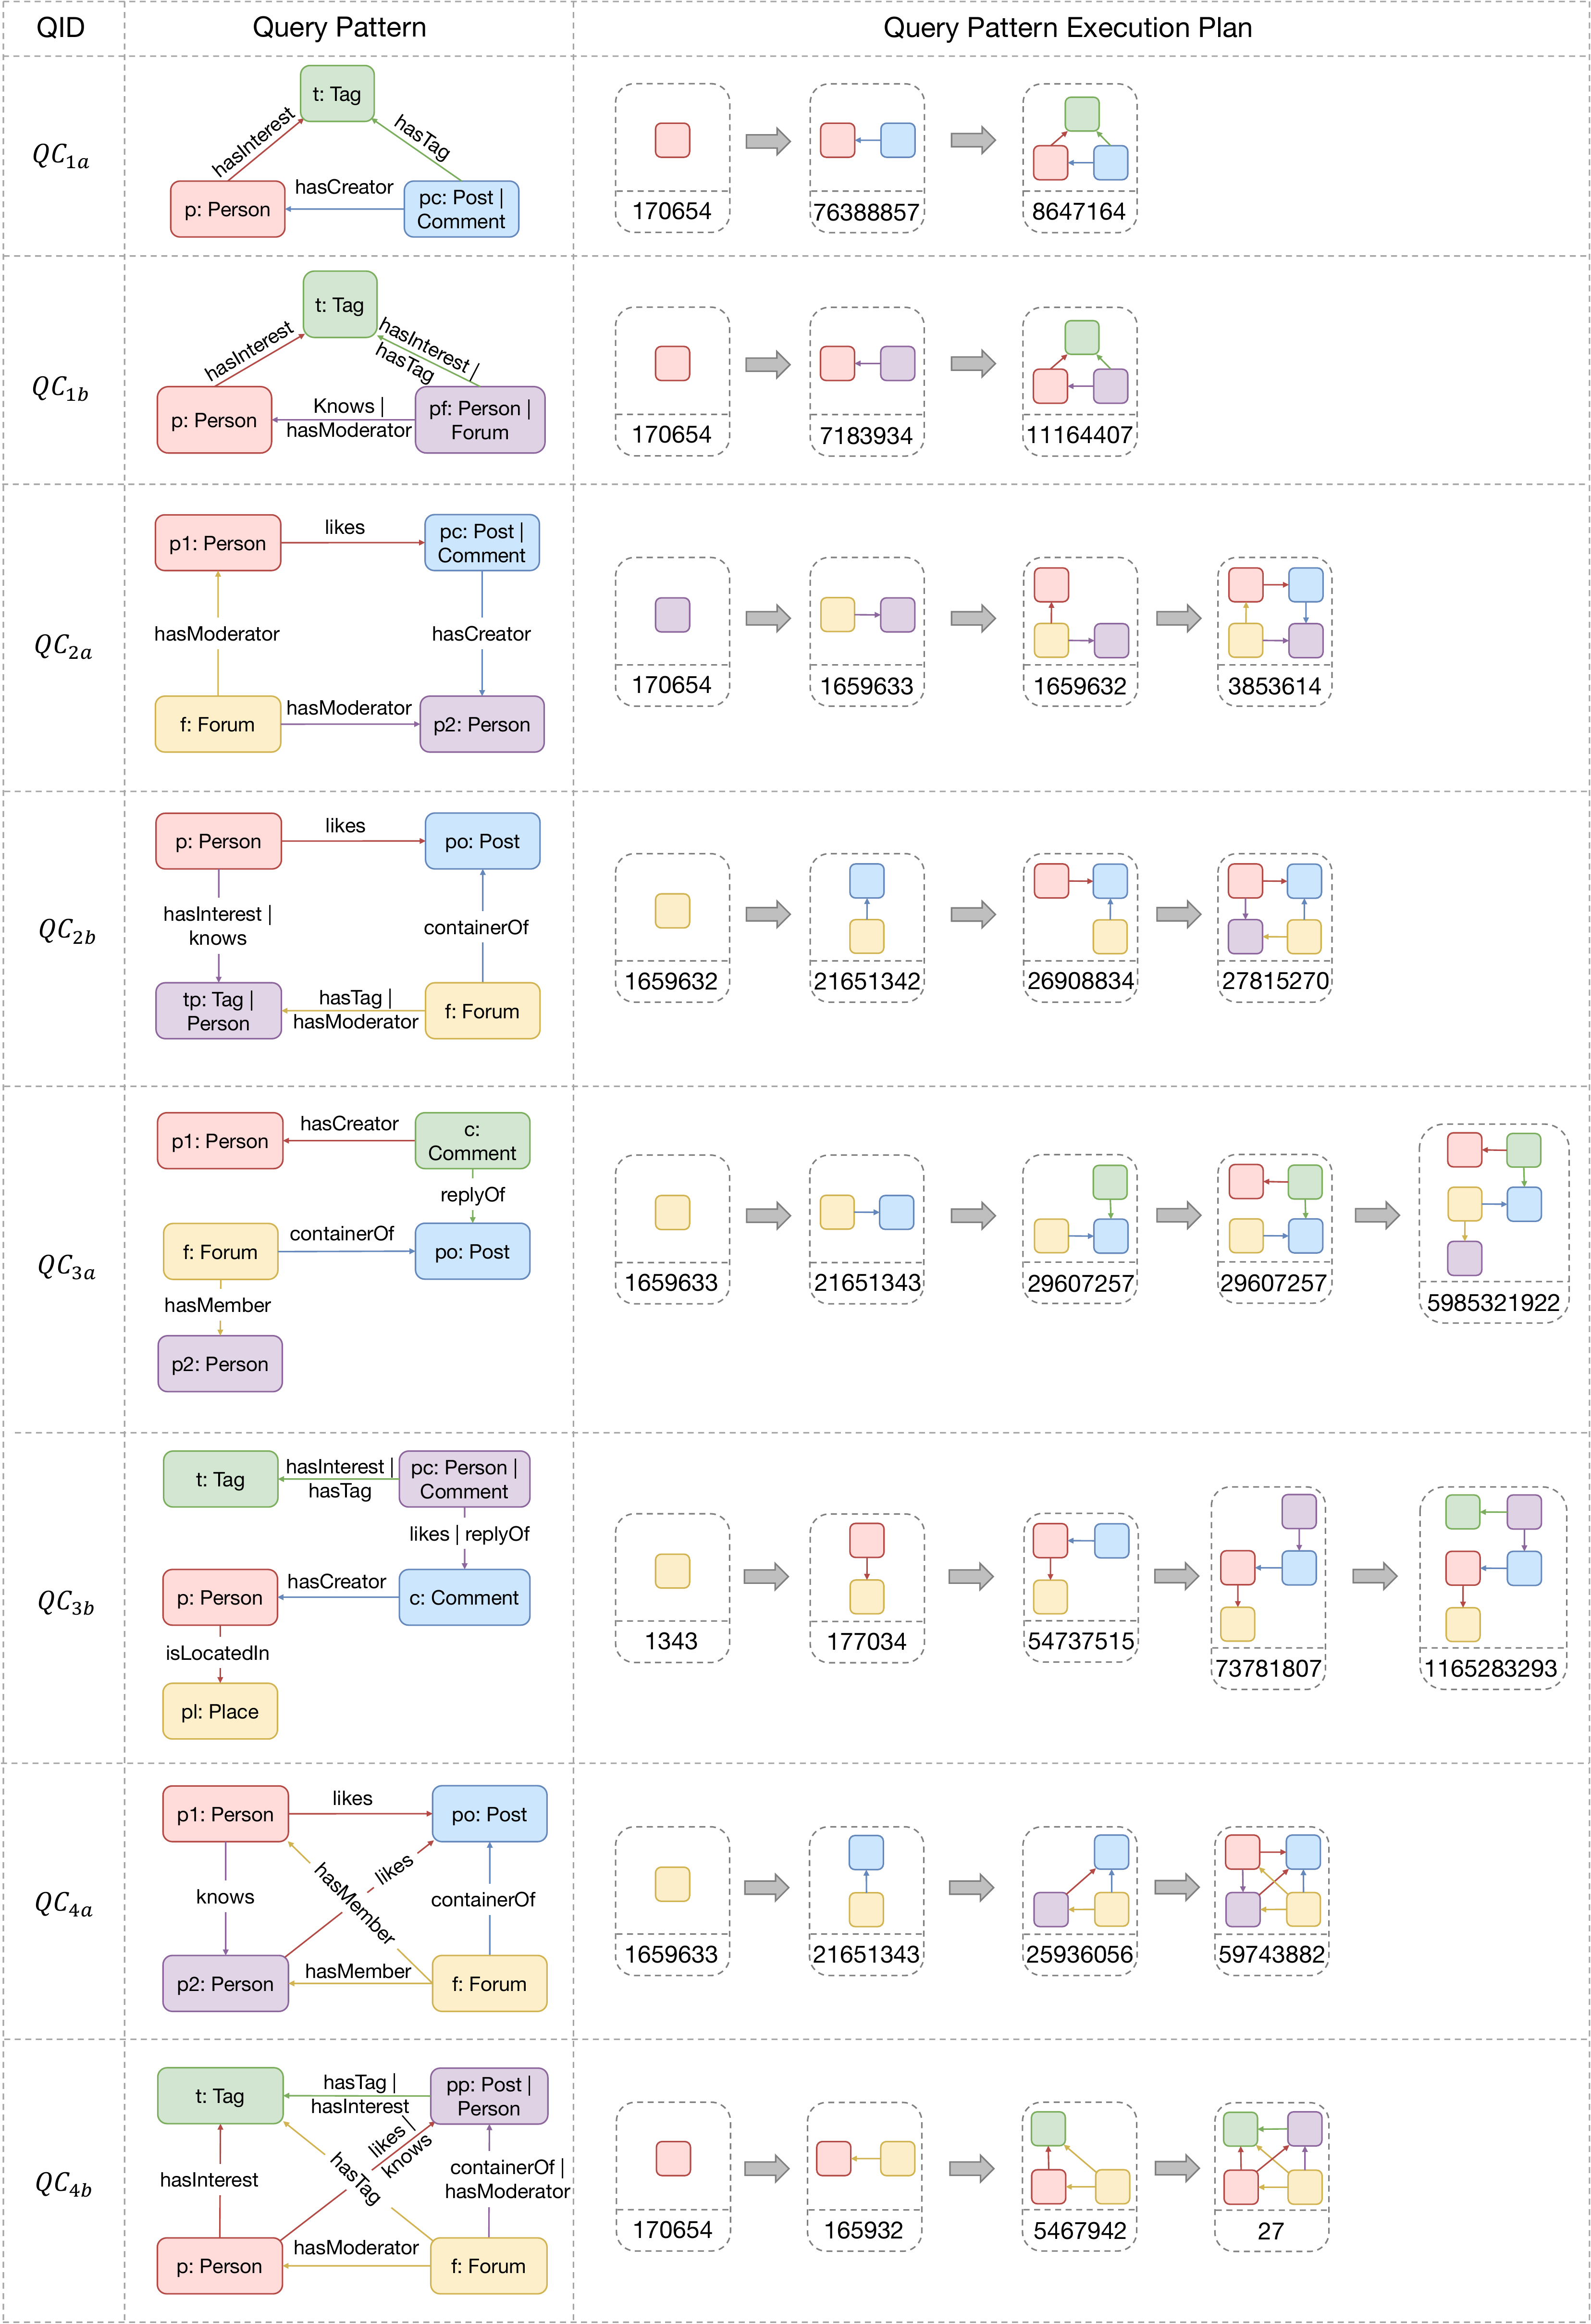}
  \caption{Optimized Execution Plans by GOpt for $Q_{c}[1\ldots 4(a|b)]$}
  \label{fig:cbo_plans}
\end{figure*}

\subsubsection{Execution Plans for Queries}
We present the execution plans for queries $QC_{1\ldots 4(a|b)}$, which have been optimized by \gopt. 
These plans are illustrated in \reffig{cbo_plans}, 
with details includes a step-by-step breakdown of the query plan generation, with a focus on the decision-making at each stage. Additionally, we specify the quantity of intermediate results generated throughout the query execution, providing insight into the efficiency and performance implications of the optimization strategies employed by \gopt.

\subsection{Intermediate Representation}
In this subsection, we provide a more detailed description for the intermediate representation (IR) used by \gopt~to capture both graph and relational operations.
The IR abstraction defines a data model $\mathcal{D}$ that describes the structure of the intermediate results during query execution,
and a set of operators $\Omega$.

The data model $\mathcal{D}$ presents a schema-like structure 
in which each data field has a name, 
denoted as a String type, 
accompanied by a designated datatype. 
The supported datatypes encompass both graph-specific datatypes and general datatypes.
Graph-specific datatypes include \textit{Vertex}, \textit{Edge}, and \textit{Path}, as shown below:
\begin{itemize}
\item \textit{Vertex} is a datatype to represent the vertices in data graph. 
It typically consists of:
\kw{ID} that serves as a unique identifier for the vertex;
\textit{type} that characterizes the vertex class;
and \textit{properties} that includes property names and property values as a set of attributes associated with the vertex's type.
\item \textit{Edge} is a datatype to represent the edges in data graph.  
It usually includes:
\kw{EID} that acts as a unique identifier for the edge, which is a triplet
that further includes \code{src\_id} and \code{dst\_id} to pinpoint the source and destination vertices;
\textit{type} that represents the edge kind, which is also a triplet
that further includes \code{src\_type} and \code{dst\_type} to specify the source and destination vertex types;
and \textit{properties} that consist of property names and property values as a set of attributes associated with the edge's type. 
\item \textit{Path} is a datatype of an array of vertices and edges that represents a sequence of connected vertices and edges in the data graph.
It is denoted as $p = [v_1, e_1, v_2, e_2, ..., v_n]$, where $v_i$ and $e_i$ are the $i$-th vertex and edge in the path respectively.
Specifically, \textit{Path} includes \kw{PID} as a unique identifier;
and a specific property of \code{length}, denoting the number of edges in the path.
\end{itemize}
General datatypes comprise \textit{Primitives} including \textit{Integer}, \textit{Float}, \textit{String} etc., and
\textit{Collections} representing a group of elements, e.g., \textit{List}, \textit{Set}, and \textit{Map}.
Notice that the properties in vertices and edges are of general datatypes. 
For instance, a vertex with \textit{type} \code{Person} may have \textit{properties} of \code{name} (\textit{String}), \code{age} (\textit{Integer}), and \code{hobbies} (\textit{List}). 

The operators in $\Omega$ operate on data tuples extracted from $\mathcal{D}$, 
and produce a new set of data tuples as a result.
The set $\Omega$ is composed of graph operators and relational operators.
The graph operators are specifically for the retrieval of graph data and include the following:
\begin{itemize}
    \eat{
    \item \scan~is to retrieve desired vertices or edges by scanning the database. 
    It has parameters of $(alias, types, [V|E])$ to indicate the alias of the scanned results, the type constraints, and the option of whether vertex or edge to scan.
    }
    \item \getvertex~is designed to retrieve vertices from the data graph.
    It has a 4-tuple $(tag, alias, types, [SRC|TGT])$ parameter to obtain the source or target vertices from the tagged edge with the specified type constraints, and output aliased results.
    If the $tag$ is unspecified (NA), it retrieves vertices from data graph.
    \item \expandedge~is to retrieve edges from the data graph.
    It has a 4-tuple $(tag, alias, types, [OUT|IN])$ parameter to expand out or in edges from the tagged vertices with the specified type constraints, and output results with alias.
    Similarly, if the $tag$ is unspecified, it retrieves edges from data graph.
    \item \expandpath~is designed to expand paths from specified source vertices.
    It has a 5-tuple $(tag, alias, expand\_base, length, opt)$ parameter.
    Similarly, the $tag$ is used to refer to the source vertices, and the $alias$ denotes to the output results.
    $expand\_base$ is a composite of \expandedge~and \getvertex,
    defining the specific logic of each hop in the path expansion.
    The $length$ indicates the number of hops in the path.
    The $opt$ is a path option, which can be ``Arbitrary'', ``Simple'', or ``Trail'', to specify that in the result paths, all vertices and edges can be duplicated, vertices cannot be duplicated, or edge cannot be duplicated, respectively.
    These path options help to manage and limit the potential for generating unbounded path results.
    \item \matchpattern~is a composite operator consists of the above three basic graph operators,
    and is employed to describe a series of operations to match a complex pattern within the data graph.
    Specifically, we use \matchstart~and \matchend~to denote the start and end of a \matchpattern.
\end{itemize}
Notice the $types$ in the graph operators denotes the type constraints, that can be either \btype, \utype, or \unionall~based on query requirements, 
to filter out desired classes of graph elements.
The $alias$ in the operators tells the backend to store intermediate results with the given alias for further reference by subsequent operations via its $tag$. 
We offer a special empty String tag to refer to the result of the immediate previous operation, 
allowing to avoid saving unnecessary data in execution.
We also allow filter conditions fused into the operates, by the optimization rules in \gopt, i.e., the \filterrule.
Additionally, in the operator of \expandpath, the hop number is a positive integer, and we will support a range of hops in the future.
The other category of operators in $\Omega$ are relational operators $\mathcal{R}$, 
includes \project, \select, \joinopr, \order, etc., which are widely used in RDBMS. 
These operators can be applied on graph-specific data as well, 
e.g., to project properties of vertices, to select edges with specific conditions, 
or to join two sub-paths into a longer one with the join key as the end vertices of the two sub-paths.
